# Supplementary material for: PREGO: online mistake detection in PRocedural EGOcentric videos
Source: arXiv:2404.01933 source file (2024-05-17)
Supplement: Supplementary file 2 [file supp_2023-11-23.tex]

% CVPR 2024 Paper Template; see https://github.com/cvpr-org/author-kit

\documentclass[10pt,twocolumn,letterpaper]{article}

%%%%%%%%% PAPER TYPE  - PLEASE UPDATE FOR FINAL VERSION
% \usepackage{cvpr}              % To produce the CAMERA-READY version
\usepackage[review]{cvpr}      % To produce the REVIEW version
% \usepackage[pagenumbers]{cvpr} % To force page numbers, e.g. for an arXiv version

% Import additional packages in the preamble file, before hyperref
\input{preamble}

% It is strongly recommended to use hyperref, especially for the review version.
% hyperref with option pagebackref eases the reviewers' job.
% Please disable hyperref *only* if you encounter grave issues, 
% e.g. with the file validation for the camera-ready version.
%
% If you comment hyperref and then uncomment it, you should delete *.aux before re-running LaTeX.
% (Or just hit 'q' on the first LaTeX run, let it finish, and you should be clear).
\definecolor{cvprblue}{rgb}{0.21,0.49,0.74}
\usepackage[pagebackref,breaklinks,colorlinks,citecolor=cvprblue]{hyperref}


\newcommand{\FG}[1]{\textcolor{orange}{FG: #1}} % Fabio
\newcommand{\GF}[1]{\textcolor{blue}{#1}} % Giovanni
\newcommand{\AF}[1]{\textcolor{cvprblue}{AF: #1}} % Antonino
\newcommand{\GD}[1]{\textcolor{Mulberry}{GD: #1}} % Guido
\newcommand{\AL}[1]{\textcolor{cyan}{AL: #1}} % Ale
\newcommand{\LS}[1]{\textcolor{PineGreen}{LS: #1}} % Luca 
\newcommand{\ED}[1]{\textcolor{brown}{ED: #1}} % Edo
\newcommand{\LP}[1]{\textcolor{green}{LP: #1}} % Leo
\newcommand{\TD}[1]{\textcolor{red}{TODO: #1}} % TODO
\DeclareRobustCommand{\myparagraph}[1]{\noindent\textbf{#1}} 

\usepackage{pifont}
\usepackage{multirow}

\newcommand*\colourcheck[1]{%
  \expandafter\newcommand\csname #1check\endcsname{\textcolor{ForestGreen}{\ding{52}}}%
}
\colourcheck{green}

\newcommand{\cmark}{\ding{51}}


%%%%%%%%% PAPER ID  - PLEASE UPDATE
\def\paperID{4850} % *** Enter the Paper ID here
\def\confName{CVPR}
\def\confYear{2024}

%%%%%%%%% TITLE - PLEASE UPDATE
\title{PREGO: online mistake detection in PRocedural EGOcentric videos\\Supplementary Materials}

%%%%%%%%% AUTHORS - PLEASE UPDATE
\author{First Author\\
Institution1\\
Institution1 address\\
{\tt\small firstauthor@i1.org}
% For a paper whose authors are all at the same institution,
% omit the following lines up until the closing ``}''.
% Additional authors and addresses can be added with ``\and'',
% just like the second author.
% To save space, use either the email address or home page, not both
\and
Second Author\\
Institution2\\
First line of institution2 address\\
{\tt\small secondauthor@i2.org}
}

\begin{document}
\maketitle

% To complement the main paper\FG{the main paper should be self-contained, so I'd be hesitant to say "we complement". Instead, we might simply say "In this supplementary material, we provide additional notes on the following implementation, quantitative and qualitative aspects:"}, we present an ablation study on various aspects of the proposed PREGO model, offering more insights into both the recognition and anticipation components, illustrating the model architecture in detail, the performance on all the errors in the video and the cost estimation for the DaVinci model. The following table of contents indicates how the supplementary material is structured.

This supplementary material provides additional notes on our work's implementation, quantitative and qualitative aspects. Specifically, we conduct an ablation study on PREGO's different elements, investigating its recognition and anticipation components. Additionally, we provide a detailed overview of the model architecture, performance metrics for all video errors, and cost estimation for the DaVinci model. The following table of contents outlines the organization of this supplementary material.

\tableofcontents

\begin{appendix}


\section{Implementation Details} \label{sec:implementation}
% PREGO encompasses two submodules: a visual module for action recognition and a Language Model for action anticipation. 

% We build our visual model upon OadTR~\cite{OadTR}, editing part of the original model to allow it to consider a larger context window. Precisely, we only preserve the encoder module, removing the decoder part, which was originally employed for step anticipation. The encoder module is composed
% \begin{itemize}
%     \item recognition branch TSN feature, architecture with encoder only with x layer. Similarly to OadTr, we used the class token.
%     \item LM are used in the anticipation branch LM are already pretrained. It takes as input ...
%     \item pytorch on quadro P6000 with Adam optimizer, batch size=128, lr = 0.0001 and weight decay = 0.0001.
%     Training time around  4 hours (4 hour and 5 minutes) 
% \end{itemize}

We utilize TSN~\cite{TSN} as the feature extractor for both Assembly-101-O and EpicTent-O, as outlined in~\cite{sener2022assembly101}. 
The visual branch comprises a Transformer Encoder with \TODO{X} encoding layers. Each layer incorporates a Multi-Head self-attention module and an Element-Wise addition module. Similarly to~\cite{OadTR}, PREGO retains the learnable task token, part of the input to the model, along with the frame features.
We preserve the original implementation shown in~\cite{touvron2023llama} for the action anticipation branch. Adjusting the temperature and output tokens hyperparameters to \TODO{0.0} aims to enforce quasi-deterministic outputs while setting \TODO{4} ensures answers of the desired length. 
Ultimately, PREGO is trained on two P6000 GPUs using the Adam optimizer, a batch size of 128, a learning rate of \(1e^-5\), and a weight decay of \(1e^-4\). The training process, facilitated by precomputed video features, typically takes approximately 4 hours.
\AL{dobbiamo discutere LLAMA2 e Davinci non discussi \textbf{MAI} nel main paper}

% Old Version
% For both Assembly-101-O and EpicTent-O, we employ TSN~\cite{TSN} as the feature extractor, as suggested in\AL{following}~\cite{sener2022assembly101}. The visual branch is then shaped as a Transformer Encoder with \TODO{X} encoding layers, each encompassing a Multi-Head self-attention and an Element-Wise addition modules. As in~\cite{OadTR}, PREGO maintains the learnable task token fed to the model together with the frame features. For the action anticipation branch, we preserve the original implementation~\cite{touvron2023llama}, setting the temperature and output tokens hyperparameters to \TODO{0.0} -to enforce quasi-deterministic outputs- and \TODO{4} -to ensure answers of the desired length-, respectively. Finally, we train PREGO on two P6000 GPUs with Adam optimizer, batch size of 128, a learning rate of \(1e^-5\), and weight decay of \(1e^-4\). With the precomputed video features, the training takes around 4 hours.
% \AL{dobbiamo discutere LLAMA2 e Davinci non discussi \textbf{MAI} nel main paper}


\section{Step Recognition} \label{sec:pictorial}

% \noindent In order to find the 

To find the best step recognition architecture in terms of mAP performance, we assess various visual models using Assembly101-O, as presented in Table \ref{tab:recognition}. Given the utilization of our new data split, it is important to highlight that these results cannot be directly compared with those obtained using Assembly101.
The experiments indicate that the Encoder-only architecture performs best regarding mAP. Furthermore, opting for this architecture significantly reduces the number of parameters compared to the original model, which is approximately three times larger. A positive correlation between mAP and the window size is observed, implying that the model gains advantages from considering more past information.
\input{Tables/supplementary/recognition}


% Seeking for the best step recognition architecture in terms of mAP performance, we evaluate in Table \ref{tab:recognition} different visual models using Assembly101-O. It is worth noting that these results are not comparable with those obtained with Assembly101 since we use our new data split.

% The experiments suggest that the Encoder-only architecture is the best for mAP. In addition to that, this choice leads to a considerable reduction of the number of parameters with respect to the original model, which is approximately three times bigger. There is a positive correlation between the mAP and the window size, suggesting that the model benefits from considering more past information.

% An Encoder-Encoder architecture was a valid alternative to the original model: here, a branch is responsible for the recognition considering all the frames in the window W ${f_{{\tau}-w}, ..., f_{\tau}}$, while the other performs the anticipation of the action in the current frame considering the frames ${f_{{\tau}-w}, ..., f_{{\tau}-1} }$. At the end of the procedure, the mean of the two branches' output is given as the final result. Unlike the previous cases, the Encoder-Encoderarchitecture reports a degradation of the mAP performance after a certain window size.



\section{All Mistake Detection} \label{sec:AMD}
\TD{experiments} \AL{work in progress} \GD{work in progress}\\
While building our new benchmark, we made a critical choice: considering procedures until they are compromised by a mistake since the split between correct Vs. mistake procedures for train and validation/test sets, respectively, does not allow for mistaken procedures to be employed in our model workflow. On the other hand, this split is required to guarantee the model adheres to the open-set mistake detection protocol. Nevertheless, this section provides the results obtained by PREGO and its competitors on the whole procedures, maintaining unaltered the above-mentioned split. In this case, the visual and language models are limited since they are unaware of all the actions registered in the videos. This is because, after an error occurs, the operator makes some operation to correct the mistaken step, which, while being labeled as \textit{``corrections"} in~\cite{sener2022assembly101}, do not appear in any of our train set procedures. Results are reported in Table~\ref{tab:together_supp}. \TODO{(...)}

\input{Tables/supplementary/together_supp}

\section{Prompt Engineering} \label{sec:prompt}
\TD{experiments}\\
Sec.~4.3 of the main paper discussed the prompt structure we leverage to query PREGO to provide the next step in a partial procedural transcript. Other choices are also possible and here we report the experiments with two other strategies, namely \textit{Toy Context} (Sec.~\ref{sec:toyctxt}) and \textit{``Supervised" prompt} (Sec.~\ref{sec:supervisedLLM}).
\subsection{Toy Context}\label{sec:toyctxt}
As reported in Sec.~4.3, we provide the LLM module of PREGO with the current sequence (the online output of the visual module) together with a context, indicating similar correct procedures to acknowledge the model about the right steps and their order in related sequences. The context procedures are defined as all the correct procedures on the same toy as the current one performed by different actors and all the correct procedures on the same kind of toy, i.e., toys with different names but with many shared subparts. We report here the experiment obtained with a slightly different choice for the context definition, where we consider as context only the procedures to assemble toys that share the same name (and hence, the same subparts) with the one the model is currently dealing with. The results are described in Table~\ref{tab:toys}, and \TODO{(...)}
\subsection{"Supervised" prompt}\label{sec:supervisedLLM}
As a further analysis, we conduct an experiment providing the LLM with a different prompt structure. Indeed, instead of feeding Llama-2\cite{touvron2023llama} with examples of correct procedures and with the current transcript, we provide examples of correct and mistaken procedures, labeling the former as ``\textit{correct}" and the latter as ``\textit{mistake - \#}", where \textit{\#} stands for the symbolic representation of the erroneous step. Right after the context, we append the current transcript as it has been detected from the visual module and question the module to label it as correct or mistake. The results of this experiment are shown in Table~\ref{tab:supervised}.~\TODO{(...)}
% \AL{l'idea è di dare come contesto al LLM sequence giuste e sbagliata, con annotazione annessa. Poi, come sequenza input, dare una sequenza e chiedere al LLM "è corretta o contiene mistake?" }


\section{Step Anticipation multiple outputs} \label{sec:prompt}
\TD{experiments}\\
\AL{esperimento tolto dal main paper. Ablation sul numero di risposte dato dal LLM. Descrescono le performance perchè scendono i TP. }

% \section{Pictorial} \label{sec:pictorial}

% Fig. \ref{fig:pictorial}

\begin{figure*}[htbp]
    \centering
    \includegraphics[width=\linewidth]{Images/pictorial_framework.pdf}
    \caption{Pictorial of the model.}
    \label{fig:pictorial}
\end{figure*}

\section{DaVinci cost estimation and performance on Epic-Tent} \label{sec:davinci}
\TD{experiments}\\
risultati incoraggianti. Contesto limitato perchè il task in epic-tent è sempre quello. Non possiamo utilizzare tutti i video per il prompt in quanto costerebbe. Lavoriamo su subset.
{
    \small
    \bibliographystyle{ieeenat_fullname}
    \bibliography{main}
}

% WARNING: do not forget to delete the supplementary pages from your submission 
% \input{sec/X_suppl}
\end{appendix}

\end{document}
