# Supplementary material for: PREGO: online mistake detection in PRocedural EGOcentric videos
Source: arXiv:2404.01933 source file (2024-05-17)
Supplement: Supplementary file 3 [file supp_2023-11-26.tex]

% CVPR 2024 Paper Template; see https://github.com/cvpr-org/author-kit

\documentclass[10pt,twocolumn,letterpaper]{article}

%%%%%%%%% PAPER TYPE  - PLEASE UPDATE FOR FINAL VERSION
% \usepackage{cvpr}              % To produce the CAMERA-READY version
\usepackage[review]{cvpr}      % To produce the REVIEW version
% \usepackage[pagenumbers]{cvpr} % To force page numbers, e.g. for an arXiv version

% Import additional packages in the preamble file, before hyperref
\input{preamble}

% It is strongly recommended to use hyperref, especially for the review version.
% hyperref with option pagebackref eases the reviewers' job.
% Please disable hyperref *only* if you encounter grave issues, 
% e.g. with the file validation for the camera-ready version.
%
% If you comment hyperref and then uncomment it, you should delete *.aux before re-running LaTeX.
% (Or just hit 'q' on the first LaTeX run, let it finish, and you should be clear).
\definecolor{cvprblue}{rgb}{0.21,0.49,0.74}
\usepackage[pagebackref,breaklinks,colorlinks,citecolor=cvprblue]{hyperref}


\newcommand{\FG}[1]{\textcolor{orange}{FG: #1}} % Fabio
\newcommand{\GF}[1]{\textcolor{blue}{#1}} % Giovanni
\newcommand{\AF}[1]{\textcolor{cvprblue}{AF: #1}} % Antonino
\newcommand{\GD}[1]{\textcolor{Mulberry}{GD: #1}} % Guido
\newcommand{\AL}[1]{\textcolor{cyan}{AL: #1}} % Ale
\newcommand{\LS}[1]{\textcolor{PineGreen}{LS: #1}} % Luca 
\newcommand{\ED}[1]{\textcolor{brown}{ED: #1}} % Edo
\newcommand{\LP}[1]{\textcolor{green}{LP: #1}} % Leo
\newcommand{\TD}[1]{\textcolor{red}{TODO: #1}} % TODO
\DeclareRobustCommand{\myparagraph}[1]{\noindent\textbf{#1}} 

\usepackage{pifont}
\usepackage{multirow}

\newcommand*\colourcheck[1]{%
  \expandafter\newcommand\csname #1check\endcsname{\textcolor{ForestGreen}{\ding{52}}}%
}
\colourcheck{green}

\newcommand{\cmark}{\ding{51}}


%%%%%%%%% PAPER ID  - PLEASE UPDATE
\def\paperID{4850} % *** Enter the Paper ID here
\def\confName{CVPR}
\def\confYear{2024}

%%%%%%%%% TITLE - PLEASE UPDATE
\title{PREGO: online mistake detection in PRocedural EGOcentric videos\\Supplementary Materials}

%%%%%%%%% AUTHORS - PLEASE UPDATE
\author{First Author\\
Institution1\\
Institution1 address\\
{\tt\small firstauthor@i1.org}
% For a paper whose authors are all at the same institution,
% omit the following lines up until the closing ``}''.
% Additional authors and addresses can be added with ``\and'',
% just like the second author.
% To save space, use either the email address or home page, not both
\and
Second Author\\
Institution2\\
First line of institution2 address\\
{\tt\small secondauthor@i2.org}
}

\begin{document}
\maketitle

% To complement the main paper\FG{the main paper should be self-contained, so I'd be hesitant to say "we complement". Instead, we might simply say "In this supplementary material, we provide additional notes on the following implementation, quantitative and qualitative aspects:"}, we present an ablation study on various aspects of the proposed PREGO model, offering more insights into both the recognition and anticipation components, illustrating the model architecture in detail, the performance on all the errors in the video and the cost estimation for the DaVinci model. The following table of contents indicates how the supplementary material is structured.

This supplementary material provides additional notes on our work's implementation, quantitative and qualitative aspects. Specifically, we conduct an ablation study on PREGO's different elements, investigating its recognition and anticipation components. Additionally, we provide a detailed overview of the model architecture, performance metrics for all video errors, and cost estimation for the DaVinci model. The following table of contents outlines the organization of this supplementary material. \AL{da aggiornare quando le sezioni sono stabilite.}

\tableofcontents

\begin{appendix}

\section{Implementation Details} \label{sec:implementation}
In this section, we discuss step recognition architecture, delve into details on symbolic reasoning, and provide insights into the hyperparameters used. 


% Old Version
% For both Assembly-101-O and EpicTent-O, we employ TSN~\cite{TSN} as the feature extractor, as suggested in\AL{following}~\cite{sener2022assembly101}. The visual branch is then shaped as a Transformer Encoder with \TODO{X} encoding layers, each encompassing a Multi-Head self-attention and an Element-Wise addition modules. As in~\cite{OadTR}, PREGO maintains the learnable task token fed to the model together with the frame features. For the action anticipation branch, we preserve the original implementation~\cite{touvron2023llama}, setting the temperature and output tokens hyperparameters to \TODO{0.0} -to enforce quasi-deterministic outputs- and \TODO{4} -to ensure answers of the desired length-, respectively. Finally, we train PREGO on two P6000 GPUs with Adam optimizer, batch size of 128, a learning rate of \(1e^-5\), and weight decay of \(1e^-4\). With the precomputed video features, the training takes around 4 hours.
% \AL{dobbiamo discutere LLAMA2 e Davinci non discussi \textbf{MAI} nel main paper}


\paragraph{Step Recognition.} \label{sec:pictorial}

% \noindent In order to find the 
% \GD{va rivisto a valle dei nuovi dati WS=(768, 1024) e aggiunto il parameter count}\\
% \AL{moved this from the first part of the implementation details. from here:}
We employ TSN~\cite{TSN} as the feature extractor for both Assembly101-O and EpicTent-O, as outlined in~\cite{sener2022assembly101}. 
% \AL{we already had the pre-extracted TSN features from \cite{sener2022assembly101}. We used the same extractor for Epic-Tent. should we mention it?}
The visual branch comprises a Transformer Encoder with 3 encoding layers. Each layer incorporates a Multi-Head self-attention module and an Element-Wise addition module. Similarly to~\cite{OadTR}, PREGO retains the learnable task token, part of the input to the model, along with the frame features. 
% \AL{:to here}

To find the best step recognition architecture in terms of mAP performance, we assess two visual models, as presented in Table~\ref{tab:recognition} and Fig.~2 of the main paper. It is worth noting that these results express the performance of the models on our proposed Assembly101-O, and they should not be directly compared with those obtained using Assembly101.
The Encoder-only architecture outperforms the original OadTR architecture for all the time window choices. In particular, the best window size for our proposed Encoder architecture, reporting the maximum mAP score of $14.45$, $10\%$ times better than OadTR. Furthermore, the Encoder-only significantly reduces the number of parameters compared to the original model, which is approximately three times larger. A positive correlation between mAP and the window size is observed for smaller window sizes, suggesting that the model gains advantages from considering more past information.
Nevertheless, after 512, we see a degradation of the mAP. By fixing the window size to 512, not only we have the best mAP, but we also reach a good trade-off between window dimension, which represents the past information available to the model, and number of first frames of a video we are not considering. In fact, if the window size is $w$, we produce an output starting from the frame $f_w$ on, effectively neglecting the possibility to find a mistake if it is located in the frames $f_0,..., f_{w-1}$ . 
% \GD{da riscrivere qui, non chiaro perché non lo consider}

The Runtime, computed on a single sample, shows the advantage of using PREGO architecture due to the strict time requirements of the online setup. In fact, it is approximately 80\% faster than the original model.

Notably, the Encoder-Decoder model underperforms the Encoder-Only for Step Recognition on Assembly101-O. We suppose that the limited size of the training data might harm the larger model, hindering the proper learning of its parameters.
% The final consideration is about the performance of the Encoder-Decoder architecture that, in principle, should be \GF{GMF: is expected to be?} better than the one offered by the Encoder only architecture. However, the limited size of the training data might harm the larger model, which can not tune all its parameters properly.

\input{Tables/supplementary/recognition}

% An Encoder-Encoder architecture was a valid alternative to the original model: here, a branch is responsible for the recognition considering all the frames in the window W ${f_{{\tau}-w}, ..., f_{\tau}}$, while the other performs the anticipation of the action in the current frame considering the frames ${f_{{\tau}-w}, ..., f_{{\tau}-1} }$. At the end of the procedure, the mean of the two branches' output is given as the final result. Unlike the previous cases, the Encoder-Encoderarchitecture reports a degradation of the mAP performance after a certain window size.

\paragraph{Symbolic Reasoning.}
We adopt Llama-2~\cite{touvron2023llama} as the LLM module for symbolic reasoning. The Llama-2 family presents three versions of the model, varying the number of parameters from 7 to 70 billion parameters. It outperforms the original Llama model by training 40\% more tokens and extending the context length to 4,000 tokens. 

% Accessible on platforms like Kaggle, it can be downloaded in various sizes, including pre-trained Chat and Code Llama models. Tailored for quick deployment as a conversational agent, Llama 2 follows a specific prompt structure with special tokens. Resources, including guides for fine-tuning, quantization, and validation, assist in setup. 

We preserve the original implementation shown in~\cite{touvron2023llama} for the action anticipation branch. Adjusting the temperature and output tokens hyperparameters to 0.6 for the former, which aims to enforce quasi-deterministic outputs, while setting the latter to 4 to ensure answers of the desired length. 

\LS{add some info on Davinci03}

\paragraph{Learning.}
% We utilize TSN~\cite{TSN} as the feature extractor for both Assembly101-O and EpicTent-O, as outlined in~\cite{sener2022assembly101}. 
% The visual branch comprises a Transformer Encoder with 3 encoding layers. Each layer incorporates a Multi-Head self-attention module and an Element-Wise addition module. Similarly to~\cite{OadTR}, PREGO retains the learnable task token, part of the input to the model, along with the frame features. \AL{here we're talking of OadTR, I'd put it in the Step Recognition paragraph}
% We preserve the original implementation shown in~\cite{touvron2023llama} for the action anticipation branch. Adjusting the temperature and output tokens hyperparameters to 0.6 for the former, which aims to enforce quasi-deterministic outputs, while setting the latter to 4 to ensure answers of the desired length.
% Ultimately, 
PREGO is trained on two P6000 GPUs using the Adam optimizer, a batch size of 128, a learning rate of \(1e^-5\), and a weight decay of \(1e^-4\). The training process, facilitated by precomputed video features at the frame level, takes approximately 4 hours.


\section{Limitations}\label{sec:AMD}

% \TD{experiments} 
% \AL{work in progress} 
% \GD{work in progress}\\
% While building our new benchmark, we made a critical choice: considering procedures until they are compromised by a mistake since the split between correct Vs. mistake procedures for train and validation/test sets, respectively, does not allow for mistaken procedures to be employed in our model workflow. On the other hand, this split is required to guarantee the model adheres to the open-set mistake detection protocol. Nevertheless, this section provides the results obtained by PREGO and its competitors on the whole procedures, maintaining unaltered the above-mentioned split. In this case, the visual and language models are limited since they are unaware of all the actions registered in the videos. This is because, after an error occurs, the operator makes some operation to correct the mistaken step, which, while being labeled as \textit{``corrections"} in~\cite{sener2022assembly101}, do not appear in any of our train set procedures. Results are reported in Table~\ref{tab:together_supp}. \TODO{(...)}

% stemming from the selected datasets and the constraints we enforce to build them \GF{GMF: It is probably better to say that there was no dataset aligned with the proposed task. hence we adapted a state of the art dataset to perform the study considering constraints given by our settings}. Firstly, it only accounts for videos until they are compromised by a mistake. This limitation stems from our training methodology, which solely focuses on error-free procedures. Hence, during inference, our model cannot predict or adapt to corrective actions or unforeseen scenarios not covered during training. Indeed, considering the complete procedures would harm the step anticipator, which relies only on correct procedures. This limitation in the training data suggests that the model may face challenges in adapting to real-world scenarios, where deviations and corrections are more frequent.

Our benchmark is the first to allow the study of online mistake detection in an open-set framework. Nevertheless, it reveals some limitations, primarily due to the fact that there was no dataset aligned with the proposed task. Hence, we adapted two recent datasets to perform the study, considering the constraints given by our settings.


Secondly, the scope of Assembly-101~\cite{sener2022assembly101}, despite encompassing numerous hours of footage, is restricted in terms of procedural diversity. With approximately 330 procedures recorded, of which only 190 are entirely correct, our learning base proves relatively narrow. This dearth of varied data challenges the model to learn and generalize across a wide range of tasks. The skew towards correct procedures further narrows the model's exposure, limiting its ability to handle the complexities of real-world tasks that often involve a mix of correct and incorrect procedures. This is even true for EpicTent~\cite{epictent}, where only 29 videos are available, all representing the same task. Consequently, the limited diversity in our benchmark datasets may hinder the model's ability to robustly adapt to a broader range of real-world procedures, where encountering both correct and incorrect steps is typical.

Thirdly, while we consider EpicTent to be included in our benchmark since it showcases open-air, goal-oriented, unscripted procedures, it is decisively different from Assembly-101. It describes a wide range of failures that only sometimes impede the completion of a procedure or require a corrective step (e.g., mistakes can be ``{\it slow}" or ``{\it search}") and are dissimilar from the mistakes belonging to the industrial procedures.

Recently, \cite{Industreal,HoloAssist2023} proposed datasets more consistent with our framework as they represent structured procedures with Egocentric views with and without errors. These datasets were unavailable when writing this work, but we propose including them in a more comprehensive benchmark in future work.

In our research, we found the limitations of existing datasets while defining the task and conducting experiments. The limitations we identified serve as a valuable starting point for developing new datasets specifically tailored to address the novel online mistake detection, laying the groundwork for future advancements in the field.
% \GF{GMF: we could say that we discovered the limitations of these dataset in doing the challenge of defining the task and performing the experiments; the limitations we are pointing out are a goot starting point to build new dataset considering the novel proposed challenge}
% \input{Tables/supplementary/together_supp}

\section{Prompt Context} \label{sec:prompt}
\input{Tables/supplementary/prompt_ablation}

% Sec.~4.3 of the main paper discusses the prompt structure we leverage to query PREGO to provide the next step in a partial procedural transcript. Other choices are also possible, and here we report the experiments with two other strategies.\\
% % , namely \textit{Toy Context} (Sec.~\ref{sec:toyctxt}) and \textit{``Supervised" prompt} (Sec.~\ref{sec:supervisedLLM}).\\
% \myparagraph{Prompt Structure:} We assess several structures for the prompt provided to the step anticipation module. For each presented sequence (both in the context or in the query part of the prompt) ...
% \\

In Sec.~4.3 of the main paper, we present the prompt structure we use to query PREGO for generating the next step in an incomplete procedural transcript. However, other prompt structures are also feasible. In this section, we report an additional ablation study on the effect of different prompts on the performance of PREGO, besides the one in Sec.~6.4 of the main paper. We examine two alternative ways of writing a prompt for the PREGO method: with a less representative context and a more elaborate one. Figure \TODO{N} illustrates the three versions of the prompt, while Table 2 compares the results of these two alternatives with the original prompt structure used in PREGO. 

The less informative prompt, labeled as ``Context-Absent" in Table 2, requests PREGO to produce the next step without providing the model with the information that the contexts are sequences and that the output required is a Symbol. The context is given as ``Input", and the next step is asked as ``Output". 

The more elaborate prompt, labeled ``Elaborate" in Table 2, has a more complex and lengthy prompt for both the context and the output. As shown in Fig N (b), the context is given with the sentence ``Given this sequence in input:", while the next step is requested with ``Complete this sequence:". 

The results show that the original prompt structure achieves the best F1 score (33.4). The other two alternatives have similar performance, both reaching an F1 score of 31.6.

We conclude that the original prompt structure is the most effective way of writing a prompt for the PREGO method, as it conveys the essential information and the objective of the task. However, the fact that the other two alternatives achieve comparable performance indicates that the Action Anticipation branch can consistently solve the problem even with different inputs.



% \myparagraph{Toy Context:}\label{sec:toyctxt}
% As reported in Sec.~4.3, we provide the LLM module of PREGO with the current sequence (the online output of the visual module) together with a context, indicating similar correct procedures to acknowledge the model about the right steps and their order in related sequences. The context procedures are defined as all the correct procedures on the same toy as the current one performed by different actors and all the correct procedures on the same kind of toy, i.e., toys with different names but many shared subparts. We report here the experiment obtained with a slightly different choice for the context definition, where we consider as context only the procedures to assemble toys that share the same name (and hence, the same subparts) with the one the model is currently dealing with. The results are described in Table~\ref{tab:symbolic}, and it can be noticed that considering within the context only the procedures on the same toy underperforms our proposed choice. This is probably because the context is significantly reduced, as the maximum number of procedures for the same task is 7, while considering diverse toys of the same kind reports a minimum number of 5  and a maximum of 24 examples.




% \subsection{"Supervised" prompt}\label{sec:supervisedLLM}
% As a further analysis, we conduct an experiment providing the LLM with a different prompt structure. Indeed, instead of feeding Llama-2\cite{touvron2023llama} with examples of correct procedures and with the current transcript, we provide examples of correct and mistaken procedures, labeling the former as ``\textit{correct}" and the latter as ``\textit{mistake - \#}", where \textit{\#} stands for the symbolic representation of the erroneous step. Right after the context, we append the current transcript as it has been detected from the visual module and question the module to label it as correct or mistake. The results of this experiment are shown in Table~\ref{tab:supervised}.~\TODO{(...)}
% \AL{l'idea è di dare come contesto al LLM sequence giuste e sbagliata, con annotazione annessa. Poi, come sequenza input, dare una sequenza e chiedere al LLM "è corretta o contiene mistake?" }


% \section{Step Anticipation multiple outputs} \label{sec:prompt}
% \TD{experiments}\\
% \AL{esperimento tolto dal main paper. Ablation sul numero di risposte dato dal LLM. Descrescono le performance perchè scendono i TP. }

% % \section{Pictorial} \label{sec:pictorial}

% % Fig. \ref{fig:pictorial}

% \begin{figure*}[htbp]
%     \centering
%     \includegraphics[width=\linewidth]{Images/pictorial_framework.pdf}
%     \caption{Pictorial of the model.}
%     \label{fig:pictorial}
% \end{figure*}

% \section{DaVinci cost estimation and performance on Epic-Tent} \label{sec:davinci}
% \TD{experiments}\\
% risultati incoraggianti. Contesto limitato perchè il task in epic-tent è sempre quello. Non possiamo utilizzare tutti i video per il prompt in quanto costerebbe. Lavoriamo su subset.
{
    \small
    \bibliographystyle{ieeenat_fullname}
    \bibliography{main}
}

% WARNING: do not forget to delete the supplementary pages from your submission 
% \input{sec/X_suppl}
\end{appendix}

\end{document}
